# Supplementary material for: Fixed-Parameter Algorithms for Computing Kemeny Scores - Theory and Practice
Source: arXiv:1001.4003 source file (2010-01-22)
Supplement: Supplementary file 1 [file appendix.tex]

%auto-ignore
\begin{center}
\begin{scriptsize}
\textbf{Properties overview}
\vspace*{1.2ex}
\begin{tabular}{c|c|c}
  property & short name & explanation \\
  \hline
  the number of votes &\#votes ($n$) & ~ \\
  the number of candidates &\#candidates ($m$) & ~ \\
  number of swaps & $w$ & The expected number of swaps per vote. \\
  swap range & $d$ & The maximum distance of two (swapped)\\
  ~ & ~ & candidates regarding to the reference vote. \\
  the number dirty pairs &\#dirty pairs ($p$) & ~ \\
  rate of dirty pairs &\%dirty pairs & How many pairs are dirty in percent. \\
  the number majority-dirty pairs &\#dirty pairs & ~ \\
  rate of majority-dirty pairs &\%dirty pairs & How many pairs are majority-dirty in percent. \\
  minimal score & min score & The minimal pairwise score as lower bound. \\
  maximal score & max score & The maximal pairwise score as upper bound. \\
  maximum range & max range & ~ \\
  average kt-distance & average kt-dist & ~ \\
  reduced candidates & red. cands. & How many candidates could be deleted \\
  ~ & ~ & by the data reduction rule. \\
\end{tabular}
  ~ \\
  The pairwise score is the subscore of the set of all candidate pairs.
\end{scriptsize}
\end{center}
\newpage

\section{Sports competitions}
\subsection{Formula One instances}
\label{Attributes of the formula one instances}
\begin{scriptsize}
\begin{center}
 \textbf{Properties of the Formula One instances}\\
 \vspace*{1.2ex}
 \begin{tabular}{c|c|c|c|c|c|c|c|c|c|c|c}
  season & \#votes & \#candi- & \#dirty & \%dirty & \#maj. & \%maj. &  min  &  max  &  max  & average & red. \\
         &         &   dates  &   pairs &   pairs &  pairs &  pairs & score & score & range & kt-dist & cands. \\
  \hline
  1961 & 8 & 9 & 36 & 100.00 & 13 & 36.11 & 96 & 192 & 8 & 15.96 & 0 \\
  1962 & 9 & 8 & 28 & 100.00 & 8 & 28.57 & 79 & 173 & 7 & 11.81 & 0 \\
  1963 & 10 & 9 & 34 & 94.44 & 12 & 33.33 & 122 & 238 & 8 & 15.20 & 1 \\
  1964 & 10 & 9 & 36 & 100.00 & 10 & 27.78 & 143 & 217 & 8 & 17.44 & 0 \\
  1965 & 10 & 7 & 19 & 90.48 & 13 & 61.90 & 56 & 154 & 6 & 7.16 & 0 \\
  1966 & 9 & 8 & 28 & 100.00 & 7 & 25.00 & 88 & 164 & 7 & 12.58 & 0 \\
  1967 & 11 & 8 & 28 & 100.00 & 13 & 46.43 & 97 & 211 & 7 & 11.53 & 0 \\
  1968 & 12 & 8 & 28 & 100.00 & 10 & 35.71 & 111 & 225 & 7 & 12.08 & 0 \\
  1969 & 11 & 6 & 15 & 100.00 & 4 & 26.67 & 61 & 104 & 5 & 6.47 & 0 \\
  1970 & 13 & 10 & 45 & 100.00 & 15 & 33.33 & 216 & 369 & 9 & 20.85 & 0 \\
  1971 & 11 & 11 & 55 & 100.00 & 21 & 38.18 & 209 & 396 & 10 & 25.05 & 0 \\
  1972 & 12 & 11 & 55 & 100.00 & 23 & 41.82 & 204 & 456 & 10 & 23.08 & 0 \\
  1973 & 15 & 12 & 66 & 100.00 & 30 & 45.45 & 306 & 684 & 11 & 27.59 & 0 \\
  1974 & 15 & 14 & 91 & 100.00 & 35 & 38.46 & 457 & 908 & 13 & 40.35 & 0 \\
  1975 & 14 & 13 & 78 & 100.00 & 31 & 39.74 & 371 & 721 & 12 & 34.82 & 0 \\
  1976 & 16 & 13 & 78 & 100.00 & 39 & 50.00 & 410 & 838 & 12 & 33.62 & 0 \\
  1977 & 17 & 13 & 78 & 100.00 & 24 & 30.77 & 475 & 851 & 12 & 35.74 & 0 \\
  1978 & 16 & 16 & 117 & 97.50 & 69 & 57.50 & 597 & 1323 & 15 & 49.77 & 0 \\
  1979 & 15 & 19 & 168 & 98.25 & 61 & 35.67 & 823 & 1742 & 18 & 73.13 & 0 \\
  1980 & 14 & 19 & 164 & 95.91 & 91 & 53.22 & 712 & 1682 & 17 & 69.09 & 1 \\
  1981 & 15 & 19 & 167 & 97.66 & 80 & 46.78 & 767 & 1798 & 18 & 69.44 & 1 \\
  1982 & 16 & 9 & 35 & 97.22 & 21 & 58.33 & 178 & 398 & 8 & 14.33 & 0 \\
  1983 & 15 & 24 & 273 & 98.91 & 117 & 42.39 & 1282 & 2858 & 23 & 116.88 & 0 \\
  1984 & 16 & 19 & 170 & 99.42 & 89 & 52.05 & 886 & 1850 & 18 & 74.28 & 0 \\
  1985 & 16 & 14 & 91 & 100.00 & 53 & 58.24 & 458 & 998 & 13 & 38.45 & 0 \\
  1986 & 16 & 21 & 207 & 98.57 & 136 & 64.76 & 965 & 2395 & 20 & 83.89 & 0 \\
  1987 & 16 & 21 & 209 & 99.52 & 121 & 57.62 & 1026 & 2334 & 20 & 87.08 & 0 \\
  1988 & 16 & 28 & 357 & 94.44 & 252 & 66.67 & 1568 & 4480 & 24 & 137.85 & 0 \\
  1989 & 16 & 26 & 289 & 88.92 & 223 & 68.62 & 1285 & 3915 & 24 & 111.34 & 0 \\
  1990 & 16 & 24 & 249 & 90.22 & 194 & 70.29 & 1090 & 3326 & 22 & 96.28 & 0 \\
  1991 & 16 & 24 & 262 & 94.93 & 173 & 62.68 & 1178 & 3238 & 21 & 100.60 & 0 \\
  1992 & 16 & 22 & 229 & 99.13 & 130 & 56.28 & 1141 & 2555 & 21 & 97.60 & 1 \\
  1993 & 16 & 18 & 151 & 98.69 & 79 & 51.63 & 775 & 1673 & 17 & 64.68 & 0 \\
  1994 & 16 & 16 & 113 & 94.17 & 62 & 51.67 & 558 & 1362 & 15 & 45.33 & 0 \\
  1995 & 17 & 16 & 120 & 100.00 & 72 & 60.00 & 611 & 1429 & 15 & 49.40 & 0 \\
  1996 & 16 & 19 & 171 & 100.00 & 106 & 61.99 & 834 & 1902 & 18 & 71.78 & 0 \\
  1997 & 17 & 18 & 153 & 100.00 & 80 & 52.29 & 849 & 1752 & 17 & 67.49 & 0 \\
  1998 & 16 & 21 & 206 & 98.10 & 146 & 69.52 & 889 & 2471 & 20 & 78.53 & 0 \\
  1999 & 16 & 19 & 167 & 97.66 & 93 & 54.39 & 847 & 1889 & 18 & 70.19 & 0 \\
  2000 & 17 & 22 & 230 & 99.57 & 124 & 53.68 & 1170 & 2757 & 21 & 94.29 & 0 \\
  2001 & 17 & 18 & 152 & 99.35 & 67 & 43.79 & 819 & 1782 & 17 & 64.22 & 1 \\
  2002 & 17 & 18 & 140 & 91.50 & 88 & 57.52 & 751 & 1850 & 17 & 59.68 & 1 \\
  2003 & 16 & 16 & 118 & 98.33 & 79 & 65.83 & 583 & 1337 & 15 & 49.47 & 0 \\
  2004 & 18 & 15 & 101 & 96.19 & 73 & 69.52 & 425 & 1465 & 14 & 33.36 & 2 \\
  2005 & 19 & 13 & 78 & 100.00 & 58 & 74.36 & 394 & 1088 & 12 & 29.05 & 0 \\
  2006 & 18 & 18 & 152 & 99.35 & 100 & 65.36 & 682 & 2072 & 17 & 54.41 & 0 \\
  2007 & 17 & 18 & 149 & 97.39 & 108 & 70.59 & 602 & 1999 & 17 & 49.91 & 0 \\
  2008 & 18 & 20 & 182 & 95.79 & 111 & 58.42 & 923 & 2497 & 19 & 71.47 & 0 \\
 \end{tabular}
\end{center}
\end{scriptsize}
\newpage
\begin{scriptsize}
\begin{center}
 \textbf{Running times (in seconds) for the Formula One instances}\\
 \vspace*{1.2ex}
 \begin{tabular}{c|c|c|c|c|c|c}
  season & \texttt{kconsens\_cands} & \texttt{kconsens\_pairs} & \texttt{kconsens\_triples} & \texttt{$4$-kconsens} & \texttt{$5$-kconsens} & \texttt{$6$-kconsens} \\
  \hline
  1961 & 0.051 & n/a & 108.461 & 32.031 & 59.121 & 147.581 \\
  1962 & 0.021 & n/a & 7.371 & 2.221 & 4.281 & 11.811 \\
  1963 & 0.041 & n/a & 68.701 & 25.711 & 48.771 & 111.531 \\
  1964 & 0.051 & n/a & n/a & 68.721 & 147.401 & n/a \\
  1965 & 0.001 & 0.651 & 0.021 & 0.001 & 0.011 & 0.021 \\
  1966 & 0.021 & n/a & 13.611 & 3.071 & 6.151 & 18.761 \\
  1967 & 0.021 & n/a & 4.201 & 0.981 & 2.231 & 5.851 \\
  1968 & 0.021 & n/a & 1.431 & 0.001 & 0.011 & 0.061 \\
  1969 & 0.001 & 0.241 & 0.111 & 0.051 & 0.071 & 0.091 \\
  1970 & 0.111 & n/a & n/a & 705.771 & n/a & n/a \\
  1971 & 0.281 & n/a & n/a & 5831.82 & n/a & n/a \\
  1972 & 0.281 & n/a & n/a & 2042 & n/a & n/a \\
  1973 & 0.861 & n/a & n/a & n/a & n/a & n/a \\
  1974 & 11.351 & n/a & n/a & n/a & n/a & n/a \\
  1975 & 2.931 & n/a & n/a & n/a & n/a & n/a \\
  1976 & 2.921 & n/a & n/a & n/a & n/a & n/a \\
  1977 & 2.931 & n/a & n/a & n/a & n/a & n/a \\
  1978 & 111.961 & n/a & n/a & n/a & n/a & 0.241 \\
  1979 & 8426.59 & n/a & n/a & n/a & n/a & n/a \\
  1980 & 1927.58 & n/a & n/a & n/a & n/a & n/a \\
  1981 & 1992.62 & n/a & n/a & n/a & n/a & n/a \\
  1982 & 0.051 & n/a & 4.811 & 0.001 & 0.631 & 0.771 \\
  1983 & a few hours & n/a & n/a & n/a & n/a & n/a \\
  1984 & 8310.57 & n/a & n/a & n/a & n/a & n/a \\
  1985 & 10.571 & n/a & n/a & n/a & n/a & n/a \\
  1986 & a few hours & n/a & n/a & n/a & n/a & n/a \\
  1987 & a few hours & n/a & n/a & n/a & n/a & n/a \\
  1988 & a few days & n/a & n/a & n/a & n/a & n/a \\
  1989 & a few days & n/a & n/a & n/a & n/a & n/a \\
  1990 & a few days & n/a & n/a & n/a & n/a & n/a \\
  1991 & a few days & n/a & n/a & n/a & n/a & n/a \\
  1992 & a few hours & n/a & n/a & n/a & n/a & n/a \\
  1993 & 1962.81 & n/a & n/a & n/a & n/a & n/a \\
  1994 & 469.821 & n/a & n/a & n/a & n/a & n/a \\
  1995 & 101.911 & n/a & n/a & n/a & n/a & n/a \\
  1996 & 8544.33 & n/a & n/a & n/a & n/a & n/a \\
  1997 & 1966.39 & n/a & n/a & n/a & n/a & n/a \\
  1998 & a few hours & n/a & n/a & n/a & n/a & n/a \\
  1999 & 8279.19 & n/a & n/a & n/a & n/a & n/a \\
  2000 & a few hours & n/a & n/a & n/a & n/a & n/a \\
  2001 & 494.791 & n/a & n/a & n/a & n/a & n/a \\
  2002 & 484.911 & n/a & n/a & n/a & n/a & n/a \\
  2003 & 114.471 & n/a & n/a & n/a & n/a & 0.201 \\
  2004 & 49.161 & n/a & n/a & n/a & n/a & 0.191 \\
  2005 & 2.821 & n/a & n/a & n/a & n/a & n/a \\
  2006 & 1929.25 & n/a & n/a & n/a & n/a & n/a \\
  2007 & 2015.77 & n/a & n/a & n/a & n/a & n/a \\
  2008 & a few hours & n/a & n/a & n/a & n/a & n/a \\
\end{tabular}
  \\Time values are not available for the search tree algorithms if test runs took more than three hours.
\end{center}
\end{scriptsize}

\newpage
\subsection{Winter sports instances}
\label{Attributes of the winter sports instances}
\begin{tiny}
\begin{center}
 \textbf{Properties of the winter sports instances}\\
 \vspace*{1.2ex}
 \begin{tabular}{c|c|c|c|c|c|c|c|c|c|c|c}
  competition & \#votes & \#candi- & \#dirty & \%dirty & \#maj. & \%maj. &  min  &  max  &  max  & average & red. \\
         &         &   dates  &   pairs &   pairs &  pairs &  pairs & score & score & range & kt-dist & cands. \\
  \hline
  biathlon team men 08/09 & 6 & 15 & 67 & 63.81 & 65 & 61.90 & 124 & 506 & 14 & 30.60 & 0 \\
  cross skiing 15km men 08/09 & 4 & 10 & 24 & 53.33 & 37 & 82.22 & 32 & 148 & 8 & 12.33 & 0 \\
  cross skiing seasons 06-09 & 4 & 23 & 192 & 75.89 & 190 & 75.10 & 255 & 757 & 19 & 107.17 & 0 \\
 \end{tabular}
\end{center}
\end{tiny}
~\\
\begin{tiny}
\begin{center}
\textbf{Running times (in seconds) for the winter sports instances}\\
\vspace*{1.2ex}
\begin{tabular}{c|c|c|c|c|c|c}
  competition & \texttt{kconsens\_cands} & \texttt{kconsens\_pairs} & \texttt{kconsens\_triples} & \texttt{$4$-kconsens} & \texttt{$5$-kconsens} & \texttt{$6$-kconsens} \\
  \hline
  biathlon team men 08/09 & 58.23 & n/a & n/a & 16.47 & 4904 & n/a \\
  cross skiing 15km men 08/09 & 0.081 & 30.311 & 0.721 & 0.001 & 0.011 & 0.021 \\
  cross skiing seasons 06-09 & a few hours & n/a & n/a & n/a & n/a & n/a \\
\end{tabular}
  \\Time values are not available for the search tree algorithms if test runs took more than two hours.
\end{center}
\end{tiny}

\newpage
\section{Randomly generated instances}
\subsection{Parameter values and running times for randomly generated instances}
\label{Parameter values and results for ramdomized instances}
\paragraph{Test series 1}~\vspace{0.15cm}~\\
We generated 10 instances with 200 votes for each parameter set.
The running-times are average running-times.
\begin{tiny}
\begin{center}
  \textbf{Running times and properties for test series 1}\\
  \vspace*{1.2ex}
  \begin{tabular}{r|l|l|l|l|l|l|l|l|l|l|l|l|l|l}
  $m=w=d$ & 4 & 5 & 6 & 7 & 8 & 9 & 10 & 11 & 12 & 13 & 14 & 15 & 16 & 17 \\
  \hline
  \texttt{kconsens\_cands} & 0.001 & 0.002 & 0.006 & 0.015 & 0.025 & 0.058 & 0.117 & 0.302 & 0.891 & 2.89 & 11.1 & 48.8 & 113 & 488 \\
  \texttt{kconsens\_pairs} & 0.001 & 0.013 & 0.469 & 43.21 & - & - & - & - & - & - & - & - & - & - \\
  \texttt{kconsens\_triples} & 0.003 & 0.017 & 0.0346 & 3.822 & 132.98 & - & - & - & - & - & - & - & - & - \\
  \texttt{4-kconsens} & 0.002 & 0.010 & 0.131 & 1.81 & 37.73 & 546.38 & - & - & - & - & - & - & - & - \\
  \# dirty pairs & 6 & 10 & 15 & 21 & 28 & 36 & 45 & 55 & 66 & 78 & 91 & 105 & 120 & 126 \\
 \end{tabular}
\end{center}
\end{tiny}
\paragraph{Test series 2}~\vspace{0.15cm}~\\
We generated instances with 14 candidates.
The running times are average running-times.
\begin{scriptsize}
\begin{center}
  \textbf{Running times (in seconds) and properties for test series 2}\\
  \vspace*{1.2ex}
  \begin{tabular}{l|l|l|l|l|l|l|l}
  $n$ & $p$ & $d$ & $w$ & \texttt{kconsens\_cands} & \texttt{kconsens\_pairs} & \texttt{kconsens\_triples} & \texttt{4-kconsens} \\
  \hline
  5 & 5 & 2 & 4 & 17.071 & 0.001 & 0.001 & 0.001 \\
  10 & 11 & 2 & 7 & 17.211 & 0.041 & 0.021 & 0.011 \\
  16 & 13 & 2 & 11 & 17.501 & 0.171 & 0.031 & 0.011 \\
  10 & 26 & 4 & 7 & 17.611 & n/a & 0.061 & 0.021 \\
  16 & 29 & 4 & 11 & 17.201 & n/a & 0.981 & 0.021 \\
  22 & 34 & 4 & 15 & 17.221 & n/a & 1.601 & 0.021 \\
  10 & 43 & 6 & 7 & 17.071 & n/a & 6.311 & 0.031 \\
  22 & 45 & 6 & 15 & 13.271 & n/a & 8.761 & 0.031 \\
  10 & 52 & 8 & 7 & 17.561 & n/a & n/a & 0.041 \\
  10 & 53 & 10 & 7 & 17.621 & n/a & n/a & 0.061 \\
  16 & 58 & 8 & 11 & 17.561 & n/a & n/a & 0.061 \\
  22 & 59 & 8 & 15 & 17.161 & n/a & n/a & n/a \\
  10 & 65 & 12 & 7 & 17.181 & n/a & n/a & n/a \\
  22 & 69 & 10 & 15 & 13.271 & n/a & n/a & n/a \\
  10 & 74 & 14 & 7 & 17.521 & n/a & n/a & n/a \\ 
  16 & 75 & 12 & 11 & 17.081 & n/a & n/a & n/a \\
  16 & 80 & 14 & 11 & 13.351 & n/a & n/a & n/a \\
  22 & 86 & 12 & 15 & 13.281 & n/a & n/a & n/a \\
 \end{tabular}
  \\Time values are not available for the search tree algorithms if test runs took more than 30 minutes.
\end{center}
\end{scriptsize}

\newpage
\section{Search engines}
\subsection{Attributes of the websearch instances}
\label{Attributes of the websearch instances}
Websearches with the search engines google, yahoo, ask, and msn with 300 search results per engine.
\begin{scriptsize}
\begin{center}
 \textbf{Properties of the websearch instances}\\
 \vspace*{1.2ex}
 \begin{tabular}{c|c|c|c|c|c|c|c|c|c|c}
  search term & \#candi- & \#dirty & \%dirty & \#maj. & \%maj. &  min  &  max  &  max  & average & red. \\
             &   dates  &   pairs &   pairs &  pairs &  pairs & score & score & range & kt-dist & cands. \\
  \hline
  affirmative+action & 22 & 101 & 43.72 & 203 & 87.88 & 129 & 795 & 16 & 54.33 & 6 \\
  alcoholism & 14 & 33 & 36.26 & 76 & 83.52 & 48 & 316 & 8 & 18.00 & 0 \\
  amusement+parks & 11 & 31 & 56.36 & 44 & 80.00 & 42 & 178 & 9 & 16.83 & 1 \\
  architecture & 17 & 53 & 38.97 & 121 & 88.97 & 68 & 476 & 11 & 27.50 & 0 \\
  bicycling & 20 & 85 & 44.74 & 162 & 85.26 & 113 & 647 & 15 & 45.83 & 4 \\
  blues & 20 & 77 & 40.53 & 158 & 83.16 & 109 & 651 & 12 & 43.00 & 3 \\
  cheese & 18 & 74 & 48.37 & 131 & 85.62 & 96 & 516 & 13 & 39.83 & 3 \\
  citrus+groves & 11 & 39 & 70.91 & 46 & 83.64 & 48 & 172 & 9 & 20.17 & 1 \\
  classical+guitar & 16 & 62 & 51.67 & 105 & 87.50 & 77 & 403 & 12 & 32.83 & 1 \\
  computer+vision & 18 & 115 & 75.16 & 116 & 75.82 & 152 & 460 & 15 & 62.83 & 1 \\
  cruises & 18 & 112 & 73.20 & 113 & 73.86 & 152 & 460 & 14 & 62.17 & 1 \\
  Death+Valley & 17 & 63 & 46.32 & 120 & 88.24 & 79 & 465 & 13 & 33.17 & 1 \\
  field+hockey & 18 & 63 & 41.18 & 130 & 84.97 & 86 & 526 & 11 & 34.50 & 0 \\
  gardening & 17 & 49 & 36.03 & 123 & 90.44 & 62 & 482 & 10 & 26.17 & 2 \\
  graphic+design & 11 & 21 & 38.18 & 49 & 89.09 & 27 & 193 & 6 & 10.67 & 0 \\
  Gulf+war & 18 & 62 & 40.52 & 129 & 84.31 & 86 & 526 & 13 & 34.17 & 2 \\
  HIV & 15 & 44 & 41.90 & 93 & 88.57 & 56 & 364 & 11 & 23.00 & 3 \\
  java & 17 & 65 & 47.79 & 119 & 87.50 & 82 & 462 & 14 & 34.50 & 4 \\
  Lipari & 6 & 4 & 26.67 & 15 & 100.00 & 4 & 56 & 3 & 1.50 & 6 \\
  lyme+disease & 20 & 81 & 42.63 & 172 & 90.53 & 99 & 661 & 13 & 42.00 & 0 \\
  mutual+funds & 13 & 30 & 38.46 & 69 & 88.46 & 39 & 273 & 7 & 15.50 & 1 \\
  National+parks & 13 & 32 & 41.03 & 73 & 93.59 & 37 & 275 & 10 & 15.67 & 6 \\
  parallel+architecture & 6 & 8 & 53.33 & 12 & 80.00 & 11 & 49 & 4 & 3.67 & 2 \\
  Penelope+Fitzgerald & 14 & 65 & 71.43 & 65 & 71.43 & 91 & 273 & 12 & 36.33 & 1 \\
  recycling+cans & 3 & 1 & 33.33 & 3 & 100.00 & 1 & 11 & 2 & 0.50 & 3 \\
  rock+climbing & 15 & 84 & 80.00 & 76 & 72.38 & 113 & 307 & 14 & 46.00 & 1 \\
  San+Francisco & 6 & 9 & 53.33 & 11 & 73.33 & 12 & 48 & 4 & 4.17 & 1 \\
  Shakespeare & 26 & 175 & 53.85 & 265 & 81.54 & 235 & 1065 & 21 & 96.17 & 2 \\
  stamp+collection & 9 & 19 & 52.78 & 31 & 86.11 & 24 & 120 & 8 & 9.17 & 3 \\
  sushi & 14 & 40 & 43.96 & 77 & 84.62 & 54 & 310 & 10 & 21.83 & 2 \\
  table+tennis & 13 & 38 & 48.72 & 68 & 87.18 & 48 & 264 & 9 & 19.83 & 2 \\
  telecommuting & 12 & 28 & 42.42 & 53 & 80.30 & 41 & 223 & 7 & 15.17 & 2 \\
  Thailand+tourism & 16 & 57 & 47.50 & 101 & 84.17 & 76 & 404 & 11 & 30.67 & 1 \\
  vintage+cars & 4 & 2 & 33.33 & 5 & 83.33 & 3 & 21 & 2 & 0.50 & 2 \\
  volcano & 20 & 98 & 51.58 & 159 & 83.68 & 129 & 631 & 17 & 53.17 & 0 \\
  zen+budism & 11 & 22 & 40.00 & 49 & 89.09 & 28 & 192 & 7 & 11.17 & 1 \\
  Zener & 14 & 54 & 59.34 & 74 & 81.32 & 71 & 293 & 13 & 29.00 & 1 \\
 \end{tabular}
\end{center}
\end{scriptsize}
\newpage
\begin{scriptsize}
\begin{center}
 \textbf{Running times (in seconds) for the websearch instances}\\
 \vspace*{1.2ex}
 \begin{tabular}{c|c|c|c|c|c|c}
  search term & \begin{tiny}\texttt{kconsens\_cands}\end{tiny} & \begin{tiny}\texttt{kconsens\_pairs}\end{tiny} & \begin{tiny}\texttt{kconsens\_triples}\end{tiny} & \begin{tiny}\texttt{$4$-kconsens}\end{tiny} & \begin{tiny}\texttt{$5$-kconsens}\end{tiny} & \begin{tiny}\texttt{$6$-kconsens}\end{tiny} \\
  \hline
  affirmative+action & 114.931 & n/a & n/a & n/a & 0.051 & 0.211 \\
  alcoholism & 10.871 & n/a & 4.161 & 0.011 & 0.021 & 0.101 \\
  amusement+parks & 0.081 & 34.501 & 0.001 & 0.011 & 0.001 & 0.041 \\
  architecture & 475.921 & n/a & n/a & 0.021 & 21.871 & 0.141 \\
  bicycling & 109.101 & n/a & n/a & n/a & 0.101 & n/a \\
  blues & 486.071 & n/a & n/a & n/a & 2.941 & n/a \\
  cheese & 49.891 & n/a & n/a & 1724.79 & 0.041 & 0.131 \\
  citrus+groves & 0.081 & n/a & 6.591 & 0.001 & 0.011 & 0.061 \\
  classical+guitar & 50.741 & n/a & n/a & 1087.12 & 0.031 & 0.281 \\
  computer+vision & 486.201 & n/a & n/a & n/a & n/a & n/a \\
  cruises & 475.591 & n/a & n/a & n/a & n/a & n/a \\
  Death+Valley & 109.531 & n/a & n/a & 16.901 & 0.041 & 0.151 \\
  field+hockey & 2060.72 & n/a & n/a & n/a & n/a & n/a \\
  gardening & 53.381 & n/a & n/a & 0.021 & 0.031 & 0.101 \\
  graphic+design & 0.261 & 15.611 & 0.081 & 0.001 & 0.011 & 0.031 \\
  Gulf+war & 117.931 & n/a & n/a & 126.071 & 0.041 & 3.021 \\
  HIV & 0.811 & n/a & 7.131 & 0.001 & 0.011 & 0.061 \\
  java & 2.821 & n/a & n/a & 73.441 & 0.021 & 0.361 \\
  Lipari & 0.001 & 0.001 & 0.001 & n/a & n/a & n/a \\
  lyme+disease & a few hours & n/a & n/a & n/a & n/a & 0.221 \\
  mutual+funds & 0.791 & n/a & 0.851 & 0.001 & 0.011 & 0.041 \\
  National+parks & 0.001 & 0.041 & 0.011 & 0.001 & 0.001 & 0.011 \\
  parallel+architecture & 0.001 & 0.001 & 0.001 & 0.001 & 0.001 & 0.001 \\
  Penelope+Fitzgerald & 2.841 & n/a & n/a & 0.031 & 136.241 & n/a \\
  recycling+cans & 0.001 & 0.001 & 0.001 & n/a & n/a & n/a \\
  rock+climbing & 11.831 & n/a & n/a & n/a & n/a & n/a \\
  San+Francisco & 0.001 & 0.001 & 0.011 & 0.001 & 0.011 & 0.011 \\
  Shakespeare & a few hours & n/a & n/a & n/a & n/a & n/a \\
  stamp+collection & 0.001 & 0.051 & 0.011 & 0.001 & 0.001 & 0.011 \\
  sushi & 0.801 & n/a & 32.461 & 0.201 & 0.221 & 0.061 \\
  table+tennis & 0.261 & n/a & 0.301 & 0.001 & 0.021 & 0.061 \\
  telecommuting & 0.091 & 0.261 & 0.021 & 0.001 & 0.011 & 0.041 \\
  Thailand+tourism & 51.261 & n/a & n/a & 4407.3 & 4109.55 & n/a \\
  vintage+cars & 0.001 & 0.001 & 0.001 & 0.001 & 0.001 & 0.001 \\
  volcano & a few hours & n/a & n/a & n/a & n/a & n/a \\
  zen+budism & 0.081 & 35.571 & 0.291 & 0.001 & 0.001 & 0.041 \\
  Zener & 2.791 & n/a & n/a & 0.011 & 0.041 & 0.101 \\
\end{tabular}
  \\Time values are not available for the search tree algorithms if test runs took more than three hours.
\end{center}
\end{scriptsize}
\newpage
Websearches with the search terms: ``hotel dublin'' ``hotels dublin'' ``rooms dublin'' ``bed dublin''  with 300 search results per engine.
Result urls are reduced to the domain to get greater instances.
\begin{scriptsize}
\begin{center}
 \textbf{Properties}\\
 \begin{tabular}{c|c|c|c|c|c|c|c|c|c|c}
  search- & \#candi- & \#dirty & \%dirty & \#maj. & \%maj. &  min  &  max  &  max  & average & red. \\
   engine &   dates  &   pairs &   pairs &  pairs &  pairs & score & score & range & kt-dist & cands. \\
  \hline
  ask & 4 & 4 & 66.67 & 5 & 83.33 & 5 & 19 & 3 & 2.17 & 2 \\
  google & 13 & 60 & 76.92 & 53 & 67.95 & 85 & 227 & 11 & 33.00 & 0 \\
  msnlive & 13 & 14 & 17.95 & 73 & 93.59 & 19 & 293 & 6 & 7.17 & 6 \\
  yahoo & 12 & 49 & 74.24 & 50 & 75.76 & 65 & 199 & 11 & 26.50 & 2 \\
 \end{tabular}
\end{center}
\end{scriptsize}
\begin{scriptsize}
\begin{center}
 \textbf{Running times (in seconds)}\\
 \begin{tabular}{c|c|c|c|c|c|c}
  search engine & \texttt{kconsens\_cands} & \texttt{kconsens\_pairs} & \texttt{kconsens\_triples} & \texttt{$4$-kconsens} & \texttt{$5$-kconsens} & \texttt{$6$-kconsens} \\
  \hline
  ask & 0.001 & n/a & n/a & 0.001 & 0.001 & 0.001 \\
  google & 2.431 & n/a & n/a & 0.051 & 0.061 & 0.101 \\
  msnlive & 0.001 & n/a & n/a & 0.001 & 0.001 & 0.021 \\
  yahoo & 0.081 & n/a & n/a & 8.121 & 5.321 & 0.121 \\
\end{tabular}
  \\Time values are not available for the search tree algorithms if test runs took more than 30 minutes.
\end{center}
\end{scriptsize}

Websearches with the search term list: Paris, London, Washington, Madrid, Berlin, Ottawa, Wien, Canberra, Peking, Prag, Moskau.
We generated one vote for each of the search engines: google, yahoo, ask, and msn.
The candidates are ranked according to the corresponding number of result pages.
\begin{scriptsize}
\begin{center}
 \textbf{Properties}\\
 \begin{tabular}{c|c|c|c|c|c|c|c|c|c|c}
  \#votes & \#candi- & \#dirty & \%dirty & \#maj. & \%maj. &  min  &  max  &  max  & average & red. \\
          &   dates  &   pairs &   pairs &  pairs &  pairs & score & score & range & kt-dist & cands. \\
  \hline
  4 & 11 & 19 & 34.55 & 46 & 83.64 & 28 & 192 & 6 & 10.33 & 0\\
 \end{tabular}
\end{center}
\end{scriptsize}
\begin{scriptsize}
\begin{center}
 \textbf{Running times (in seconds)}\\
 \begin{tabular}{c|c|c|c|c|c}
  \texttt{kconsens\_cands} & \texttt{kconsens\_pairs} & \texttt{kconsens\_triples} & \texttt{$4$-kconsens} & \texttt{$5$-kconsens} & \texttt{$6$-kconsens} \\
  \hline
  0.231 & 3.501 & 0.001 & 0.001 & 0.001 & 0.0041 \\
\end{tabular}
\end{center}
\end{scriptsize}
